# Supplementary material for: Combining pair-density functional theory and variational two-electron reduced-density matrix methods
Source: arXiv:1810.00753 ancillary file (2018-12-07)
Supplement: Supplementary file 1 [file SuppInfo.pdf]

# Supporting Information: Combining pair-density functional theory and variational two-electron reduced-density matrix methods

Mohammad Mostafanejad and A. Eugene DePrince III*

*Department of Chemistry and Biochemistry, Florida State University, Tallahassee, FL 32306-4390*

E-mail: deprince@chem.fsu.edu

# 1 Active space specification

The details of the full-valence active spaces used within multireference computations on a set of main-group divalent radicals are presented in Table S1. The same details for computations on $N_2$, $H_2O$ and $CN^-$ are can be found in Table S1. For the $D_{2h}$ and $C_{2v}$ point groups, the irreducible representations are ordered as $[A_g, B_{1g}, B_{2g}, B_{3g}, A_u, B_{1u}, B_{2u}, B_{3u}]$ and $[A_1, A_2, B_1, B_2]$, respectively.

Table S1: Full-valence active space specifications.

| Test Species | point group | $(n_e, n_o)$ | orbital symmetries | molecular orbitals |
|---|---|---|---|---|
| $OH^+$ | $C_{2v}$ | ( 6, 5 ) | [ 3, 0, 1, 1 ] | $\sigma_{\text{O–H}}, \sigma^*_{\text{O–H}}, 2p_{x\text{O}}, 2p_{y\text{O}}, 2p_{z\text{O}}$ |
| O | $D_{2h}$ | ( 6, 4 ) | [ 1, 0, 0, 0, 0, 1, 1, 1 ] | $2s, 2p_x, 2p_y, 2p_z$ |
| NH | $C_{2v}$ | ( 6, 5 ) | [ 3, 0, 1, 1 ] | $\sigma_{\text{N–H}}, \sigma^*_{\text{N–H}}, 2p_{x\text{N}}, 2p_{y\text{N}}, 2p_{z\text{N}}$ |
| NF | $C_{2v}$ | ( 12, 8 ) | [ 4, 0, 2, 2 ] | $\sigma_{2s}, \sigma^*_{2s}, \sigma_{2p}, \sigma^*_{2p}, 2(\pi, \pi^*)$ |
| C | $D_{2h}$ | ( 4, 4 ) | [ 1, 0, 0, 0, 0, 1, 1, 1 ] | $2s, 2p_x, 2p_y, 2p_z$ |
| $NH_2{}^+$ | $C_{2v}$ | ( 6, 6 ) | [ 3, 0, 2, 1 ] | $2(\sigma_{\text{N–H}}, \sigma^*_{\text{N–H}}), 2p_{z\text{N}}, n_{\text{N}}$ |
| $O_2$ | $D_{2h}$ | ( 12, 8 ) | [ 2, 0, 1, 1, 0, 2, 1, 1 ] | $\sigma_{2s}, \sigma^*_{2s}, \sigma_{2p}, \sigma^*_{2p}, 2(\pi, \pi^*)$ |
| Si | $D_{2h}$ | ( 4, 4 ) | [ 1, 0, 0, 0, 0, 1, 1, 1 ] | $3s, 3p_x, 3p_y, 3p_z$ |
| $CH_2$ | $C_{2v}$ | ( 6, 6 ) | [ 3, 0, 2, 1 ] | $2(\sigma_{\text{C–H}}, \sigma^*_{\text{C–H}}), 2p_{z\text{C}}, n_{\text{C}}$ |
| $PH_2{}^+$ | $C_{2v}$ | ( 6, 6 ) | [ 3, 0, 2, 1 ] | $2(\sigma_{\text{P–H}}, \sigma^*_{\text{P–H}}), 2p_{z\text{P}}, n_{\text{P}}$ |
| $SiH_2$ | $C_{2v}$ | ( 6, 6 ) | [ 3, 0, 2, 1 ] | $2(\sigma_{\text{Si–H}}, \sigma^*_{\text{Si–H}}), 2p_{z\text{Si}}, n_{\text{Si}}$ |
| $H_2CC$ | $C_{2v}$ | ( 10, 10 ) | [ 5, 0, 3, 2 ] | $2(\sigma_{\text{C–H}}, \sigma^*_{\text{C–H}}), \sigma_{\text{C–C}}, \sigma^*_{\text{C–C}}, \pi_{\text{C–C}}, \pi^*_{\text{C–C}}, 2p_{\text{C}}, n_{\text{C}}$ |
| $CF_2$ | $C_{2v}$ | ( 18, 12 ) | [ 5, 1, 2, 4 ] | $2(2s_{\text{F}}), 4(2p_{\text{F}}), 2(\sigma_{\text{C–F}}, \sigma^*_{\text{C–F}}), 2p_{\text{C}}, n_{\text{C}}$ |

Table S2: Full-valence active space specifications.

| Test Species | point group | $(n_e, n_o)$ | orbital symmetries | molecular orbitals |
|---|---|---|---|---|
| $N_2$ | $D_{2h}$ | ( 10, 8 ) | [ 2, 0, 1, 1, 0, 2, 1, 1 ] | $\sigma_{2s}, \sigma^*_{2s}, \sigma_{2p}, \sigma^*_{2p}, 2(\pi, \pi^*)$ |
| $H_2O$ | $C_{2v}$ | ( 8, 6 ) | [ 3, 0, 1, 2 ] | $\sigma_{\text{H–H}}, \sigma^*_{\text{H–H}}, 2s_{\text{O}}, 2p_{x\text{O}}, 2p_{y\text{O}}, 2p_{z\text{O}}$ |
| $CN^-$ | $C_{2v}$ | ( 10, 8 ) | [ 4, 0, 2, 2 ] | $\sigma_{2s}, \sigma^*_{2s}, \sigma_{2p}, \sigma^*_{2p}, 2(\pi, \pi^*)$ |

# 2 Singlet/triplet energy gaps for non-conjugated main-group divalent radicals

Table S3 provides errors in the calculated singlet/triplet energy gaps of a set of non-conjugated main-group divalent radicals, as compared to experimentally obtained values.

Table S3: Errors in singlet/triplet energy splittings ($\Delta E_{\text{S-T}}$, kcal mol$^{-1}$) calculated using a full-valence active space and the aug-cc-pVQZ basis set.

| Method | reference | $OH^+$ | O | NH | NF | C | $NH_2^+$ | $O_2$ | Si | $CH_2$ | $PH_2^+$ | $SiH_2$ | $H_2CC$ | $CF_2$ | MAE[a] | MAX[b] | RMSE[c] |
|---|---|---|---|---|---|---|---|---|---|---|---|---|---|---|---|---|---|
| CASSCF | CI | 6.8 | 4.9 | 7.8 | 3.7 | 5.8 | -0.5 | -1.3 | 4.9 | 1.0 | -0.1 | 2.6 | 9.2 | 0.2 | 3.7 | 9.2 | 4.8 |
| v2RDM-CASSCF | PQG | 6.8 | 4.9 | 7.7 | 3.3 | 5.8 | -3.4 | -3.9 | 4.9 | -1.2 | -1.6 | 0.8 | 3.3 | -1.6 | 3.8 | 7.7 | 4.3 |
| v2RDM-CASSCF | PQG+T2 | 6.8 | 4.9 | 7.8 | 3.5 | 5.7 | -0.6 | -1.6 | 4.9 | 1.0 | -0.1 | 2.6 | 8.9 | 0.0 | 3.7 | 8.9 | 4.7 |
| CASPT2[d] | CI | 0.8 | -1.2 | 0.5 | -2.7 | -2.0 | 2.2 | 8.6 | -1.8 | 2.0 | 0.2 | 1.0 | 4.5 | 7.4 | 2.7 | 8.6 | 3.7 |
| CASPT2-0[d] | CI | 1.4 | -0.2 | 1.1 | -2.2 | -0.2 | 4.0 | 12.3 | -0.4 | 4.1 | 2.7 | 3.3 | 6.9 | 9.3 | 3.7 | 12.3 | 5.1 |
| tPBE[d] | CI | -16.3 | -15.3 | -10.6 | -11.5 | -0.8 | -4.3 | 0.5 | -2.7 | -1.9 | -2.6 | -0.7 | -0.8 | 3.6 | 5.5 | 16.3 | 7.8 |
| tBLYP[d] | CI | -17.2 | -16.1 | -11.7 | -12.0 | -2.3 | -8.3 | -0.9 | -4.1 | -5.7 | -5.4 | -3.9 | -6.2 | 0.4 | 7.2 | 17.2 | 9.0 |
| ftPBE[d] | CI | -26.1 | -19.0 | -18.5 | -17.9 | -10.9 | -5.2 | -3.9 | -7.0 | -3.0 | -2.9 | -1.4 | -1.2 | 7.2 | 9.6 | 26.1 | 12.4 |
| ftBLYP[d] | CI | -28.4 | -21.4 | -21.1 | -19.3 | -14.1 | -9.8 | -5.3 | -10.2 | -7.7 | -6.9 | -5.3 | -7.1 | 3.5 | 12.3 | 28.4 | 14.4 |
| tPBE | PQG | -16.1 | -15.2 | -10.3 | 7.9 | -0.4 | -4.2 | -0.3 | -2.6 | -1.7 | -1.2 | 0.3 | 0.5 | 2.7 | 4.9 | 16.1 | 7.3 |
| tBLYP | PQG | -17.1 | -16.1 | -11.5 | 5.2 | -2.0 | -8.0 | -1.6 | -4.1 | -5.5 | -4.0 | -2.7 | -4.2 | -0.3 | 6.3 | 17.1 | 8.2 |
| ftPBE | PQG | -27.4 | -19.3 | -18.9 | 8.3 | -10.4 | -4.9 | -4.4 | -7.0 | -2.9 | -1.3 | 0.0 | 0.2 | 6.1 | 8.5 | 27.4 | 11.8 |
| ftBLYP | PQG | -29.7 | -21.7 | -21.5 | 5.3 | -13.8 | -9.4 | -5.7 | -10.1 | -7.5 | -5.2 | -3.6 | -5.1 | 2.6 | 10.9 | 29.7 | 13.6 |
| tPBE | PQG+T2 | -16.2 | -15.1 | -10.5 | -11.4 | -0.7 | -4.0 | 0.7 | -2.7 | -1.7 | -2.5 | -0.5 | -0.9 | 3.7 | 5.4 | 16.2 | 7.7 |
| tBLYP | PQG+T2 | -17.1 | -15.9 | -11.7 | -11.9 | -2.2 | -8.0 | -0.6 | -4.1 | -5.6 | -5.3 | -3.7 | -6.2 | 0.5 | 7.1 | 17.1 | 8.9 |
| ftPBE | PQG+T2 | -27.4 | -19.1 | -19.2 | -17.8 | -10.9 | -4.8 | -3.6 | -7.0 | -2.9 | -2.7 | -1.2 | -1.3 | 7.4 | 9.7 | 27.4 | 12.7 |
| ftBLYP | PQG+T2 | -29.7 | -21.6 | -21.9 | -19.2 | -14.2 | -9.4 | -5.0 | -10.2 | -7.6 | -6.7 | -5.1 | -7.2 | 3.6 | 12.4 | 29.7 | 14.7 |
| $\Delta E_{\text{S-T}}^{\text{expt}}$[d] | | 50.5 | 45.4 | 35.9 | 34.3 | 29.1 | 29.0 | 22.6 | 17.3 | 9.0 | -17.0 | -21.0 | -48.6 | -56.6 | – | – | – |

[a] mean absolute error.
[b] maximum absolute error.
[c] root mean square error.
[d] From Ref. 1

# 3 Potential energy curves generated using the PQG+T2 $N$-representability conditions

Potential energy curves for $N_2$, $H_2O$ and $CN^-$ computed using reduced-density matrices that satisfy the two-particle (PQG)[2] and partial three-particle (T2)[3,4] $N$-representability conditions are provided in Figs. S1, S2 and S3, respectively. Every pair of panels at the top of each quartet refers to the results of translated functionals while the bottom pairs show those corresponding to fully-translated functionals. The right-hand side panels show PECs that are shifted such that energies at $R = 3.0$ Å are zero $E_h$.

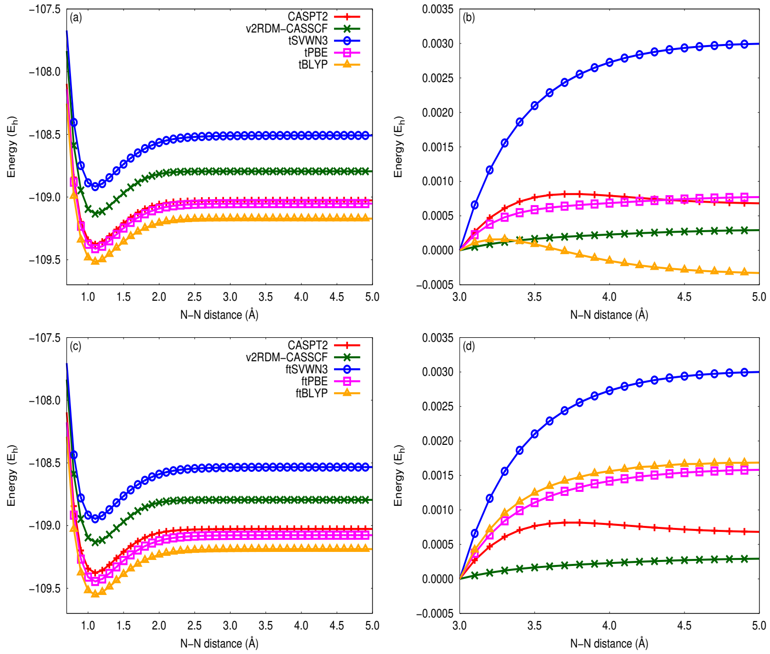


Figure S1: Potential energy curves for the dissocation of $N_2$ within the cc-pVTZ basis set [(a), (c)], as well as their behavior in the limit of dissociation [(b), (d)]. RDMs from v2RDM-CASSCF employed within v2RDM-CASSCF-PDFT satisfy the PQG and T2 $N$-representability conditions. Results are provided using both the translated [(a), (b)] and fully-translated [(c), (d)] v2RDM-CASSCF-PDFT schemes.

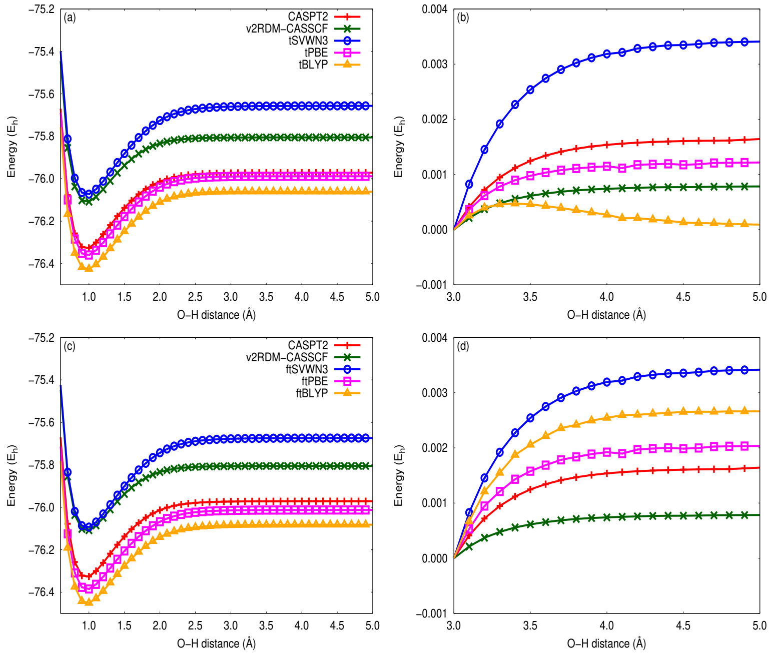


Figure S2: Potential energy curves for the symmetric dissocation of $H_2O$ within the cc-pVTZ basis set [(a), (c)], as well as their as their behavior in the limit of dissociation [(b), (d)]. RDMs from v2RDM-CASSCF employed within v2RDM-CASSCF-PDFT satisfy the PQG and T2 $N$-representability conditions. Results are provided using both the translated [(a), (b)] and fully-translated [(c), (d)] v2RDM-CASSCF-PDFT schemes.

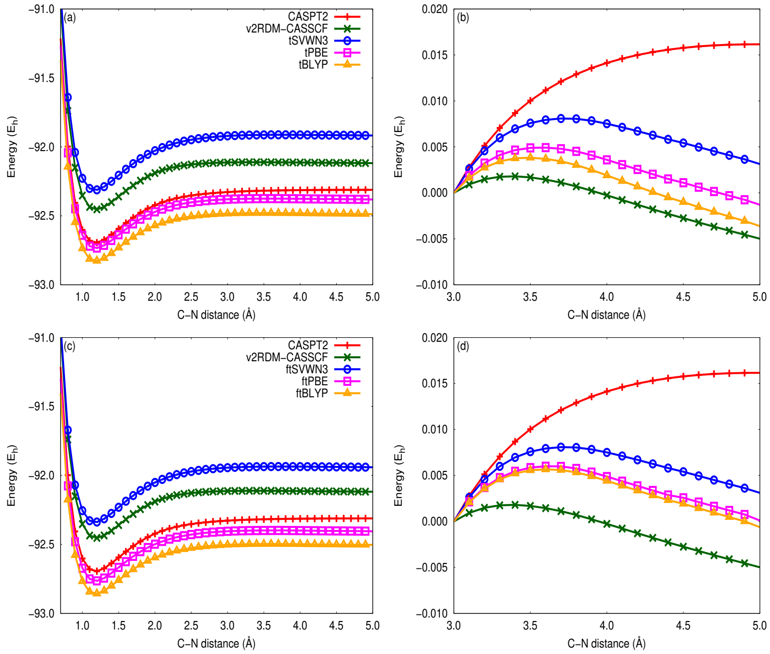


Figure S3: Potential energy curves for the dissocation of $CN^-$ within the cc-pVTZ basis set [(a), (c)], as well as as their behavior in the limit of dissociation [(b), (d)]. RDMs from v2RDM-CASSCF employed within v2RDM-CASSCF-PDFT satisfy the PQG and T2 $N$-representability conditions. Results are provided using both the translated [(a), (b)] and fully-translated [(c), (d)] v2RDM-CASSCF-PDFT schemes.

# 4 Singlet/triplet energy gaps for linear polyacene molecules

Table S4 presents singlet/triplet energy gaps for linear polyacene molecules computed using v2RDM-CASSCF and v2RDM-CASSCF-PDFT within the cc-pVTZ basis set. The experimental data are taken from Refs. 5–12.

Table S4: Singlet/triplet energy gaps (kcal $mol^{-1}$) of the linear polyacene series. The label $k$ refers to the number of fused benzene rings that comprise the molecule.

| $k$ | v2RDM-CASSCF | tSVWN3 | tPBE | tBLYP | ftSVWN3 | ftPBE | ftBLYP | Experiment |
|---|---|---|---|---|---|---|---|---|
| 2 | 63.20 | 68.58 | 66.36 | 65.75 | 69.48 | 65.12 | 65.25 | 61.0 |
| 3 | 44.52 | 47.35 | 46.04 | 45.76 | 47.95 | 45.16 | 45.39 | 43.1 |
| 4 | 31.79 | 32.39 | 31.65 | 31.53 | 32.76 | 31.12 | 31.35 | 29.3 |
| 5 | 23.39 | 22.02 | 21.62 | 21.56 | 22.24 | 21.39 | 21.56 | 19.8 |
| 6 | 18.08 | 15.29 | 15.06 | 15.01 | 15.42 | 15.05 | 15.15 | – |
| 7 | 14.79 | 11.44 | 11.27 | 11.22 | 11.52 | 11.37 | 11.42 | – |
| 8 | 12.66 | 9.32 | 9.16 | 9.11 | 9.37 | 9.29 | 9.32 | – |
| 9 | 11.16 | 8.27 | 8.10 | 8.04 | 8.31 | 8.21 | 8.22 | – |
| 10 | 10.01 | 7.40 | 7.24 | 7.19 | 7.44 | 7.34 | 7.35 | – |
| 11 | 9.05 | 6.78 | 6.62 | 6.57 | 6.82 | 6.71 | 6.72 | – |
| 12 | 8.21 | 5.99 | 5.84 | 5.79 | 6.02 | 5.94 | 5.94 | – |

# References


(1) Bao, J. L.; Sand, A.; Gagliardi, L.; Truhlar, D. G. Correlated-Participating-Orbitals Pair-Density Functional Method and Application to Multiplet Energy Splittings of Main-Group Divalent Radicals. *J. Chem. Theory Comput.* **2016**, *12*, 4274–4283.

(2) Garrod, C.; Percus, J. K. Reduction of the N-particle variational problem. *J. Math. Phys.* **1964**, *5*, 1756–1776.

(3) Zhao, Z.; Braams, B. J.; Fukuda, M.; Overton, M. L.; Percus, J. K. The reduced density matrix method for electronic structure calculations and the role of three-index representability conditions. *J. Chem. Phys.* **2004**, *120*, 2095–2104.

(4) Erdahl, R. M. Representability. *Int. J. Quantum Chem.* **1978**, *13*, 697–718.

(5) Birks, J. B. *Photophysics of aromatic molecules*; Wily-Interscience: London, 1970.

(6) Schiedt, J.; Weinkauf, R. Photodetachment photoelectron spectroscopy of mass selected anions: anthracene and the anthracene-H 2 O cluster. *Chem. Phys. Lett.* **1997**, *266*, 201–205.

(7) Angliker, H.; Rommel, E.; Wirz, J. Electronic spectra of hexacene in solution (ground state. Triplet state. Dication and dianion). *Chem. Phys. Lett.* **1982**, *87*, 208–212.

(8) Sabbatini, N.; Indelli, M. T.; Gandolfi, M. T.; Balzani, V. Quenching of singlet and triplet excited states of aromatic molecules by europium ions. *J. Phys. Chem.* **1982**, *86*, 3585–3591.

(9) Burgos, J.; Pope, M.; Swenberg, C. E.; Alfano, R. R. Heterofission in pentacene-doped tetracene single crystals. *Phys. Status Solidi B* **1977**, *83*, 249–256.

(10) Mondal, R.; Tönshoff, C.; Khon, D.; Neckers, D. C.; Bettinger, H. F. Synthesis, Stability, and Photochemistry of Pentacene, Hexacene, and Heptacene: A Matrix Isolation Study. *J. Am. Chem. Soc.* **2009**, *131*, 14281–14289.

(11) Tönshoff, C.; Bettinger, H. Photogeneration of Octacene and Nonacene. *Angew. Chem. Int. Ed.* **2010**, *49*, 4125–4128.

(12) Zade, S.; Bendikov, M. Heptacene and Beyond: The Longest Characterized Acenes. *Angew. Chem. Int. Ed.* **2010**, *49*, 4012–4015.
